# Supplementary material for: PerfGen: Automated Performance Benchmark Generation for Big Data Analytics
Source: arXiv:2412.04687 source file (2024-12-06)
Supplement: Supplementary file 1 [file metrics.tex]

% \begin{minipage}{\linewidth}
\begin{lstlisting}[language=Scala,label={appendix:metrics}]
package edu.ucla.cs.hybridfuzz.metrictemplate

import edu.ucla.cs.hybridfuzz.observers.PerfMetricsStats
import edu.ucla.cs.hybridfuzz.util.HFLogger

sealed trait Metric extends HFLogger {

 def computeColl(stats: Traversable[PerfMetricsStats]): Traversable[Long]

  // Optional reset function in case anything needs to be cleaned up - does nothing by default.
  def clear(): Unit = {}

  def isDataSkew: Boolean
  def isRuntimeSkew: Boolean

}

case class CustomMetric(computeFn: Traversable[PerfMetricsStats] => Traversable[Long], clearFn: Option[() => Unit] = None,
                        override val isDataSkew: Boolean = false, override val isRuntimeSkew: Boolean = false,
                        description: Option[String] = None) extends Metric {
  override def computeColl(stats: Traversable[PerfMetricsStats]): Traversable[Long] = computeFn(stats)

  override def clear(): Unit = clearFn.foreach(_()) // call the function if it's defined, otherwise does nothing.

  override def toString: String = description.map(s => s"${getClass.getSimpleName}($s)}").getOrElse(super.toString)

}

object Metrics {
  private case class PerfStatsMetric(accessorFn: PerfMetricsStats => Long, name: String,
                                     override val isDataSkew: Boolean = false, override val isRuntimeSkew: Boolean = false) extends Metric {
    final def computeColl(stats: Traversable[PerfMetricsStats]): Traversable[Long] = stats.map(accessorFn)

    override def toString: String = s"${getClass.getSimpleName}($name)}"
  }

  val Runtime: Metric = PerfStatsMetric(_.runtime, "Runtime", isRuntimeSkew = true)
  val GC: Metric = PerfStatsMetric(_.gcTime, "GC")
  val PeakMemory: Metric = PerfStatsMetric(_.peakExecMem, "PeakMemory")
  val InputRecords: Metric = PerfStatsMetric(_.inputReadRecords, "InputRecords", isDataSkew = true)
  val OutputRecords: Metric = PerfStatsMetric(_.outputWrittenRecords, "OutputRecords", isDataSkew = true)
  val ShuffleReadRecords: Metric = PerfStatsMetric(_.shuffleReadRecords, "ShuffleReadRecords", isDataSkew = true)
  val ShuffleWriteRecords: Metric = PerfStatsMetric(_.shuffleWriteRecords, "ShuffleWriteRecords", isDataSkew = true)
  val ShuffleReadBytes: Metric = PerfStatsMetric(_.shuffleReadBytes, "ShuffleReadBytes", isDataSkew = true)
  val ShuffleWrittenBytes: Metric = PerfStatsMetric(_.shuffleWrittenBytes, "ShuffleWrittenBytes", isDataSkew = true)

  def customMetric(computeFn: Traversable[PerfMetricsStats] => Traversable[Long], clearFn: Option[() => Unit] = None,
                   isDataSkew: Boolean = false, isRuntimeSkew: Boolean = false, description: Option[String] = None): Metric = {
    CustomMetric(computeFn, clearFn, isDataSkew, isRuntimeSkew, description)
  }
}

\end{lstlisting}
% \end{minipage}
