# Supplementary material for: PerfGen: Automated Performance Benchmark Generation for Big Data Analytics
Source: arXiv:2412.04687 source file (2024-12-06)
Supplement: Supplementary file 2 [file mutation_fns.tex]

\begin{lstlisting}[language=Scala,label={appendix:mutation_fns}]
package edu.ucla.cs.hybridfuzz.phase.mutations

import edu.ucla.cs.hybridfuzz.rddhybrid.{HybridRDD, LocalPartition, Partitions}
import edu.ucla.cs.hybridfuzz.util.{HFLogger, WeightedSampler}

import scala.reflect.{ClassTag, classTag}
import scala.util.Random

// New trait definition to separate fuzzing logic (eg. seed input management) from individual mutation definitions.
// While high-level, in practice it's generally easier to use the Partition-based one for direct data type access
trait MutationFn[T] {
  def mutate(input: HybridRDD[T]): HybridRDD[T]
}

object MutationFn {
  // Logging utility, but it would be better to standardize somewhere else...
  var mostRecent: Option[MutationFn[_]] = None
}

// Primary trait for definitions, as it allows direct access to underlying data types.
trait PartitionsBasedMutationFn[T] extends MutationFn[T] with HFLogger {
  logEnabled = false

  override final def mutate(input: HybridRDD[T]): HybridRDD[T] = {
    val mutatedPartitions = mutatePartitions(input.collectAsPartitions())
    HybridRDD(mutatedPartitions)(input.ctOutput)
  }

  // Partitions is an alias for Array[List[T]], for various serialization/management purposes
  def mutatePartitions(partitions: Partitions[T]): Partitions[T]

}

// TABLE MAPPING: ReplaceRandomRecord
abstract class RandomRecordMutationFn[T: ClassTag] extends PartitionsBasedMutationFn[T] {
  override final def mutatePartitions(partitions: Partitions[T]): Partitions[T] = {
    // Utility function to randomly select a random record from a collection of partitions
    import DataFuzzer.PartitionsRecordReplacer
    /* Code reproduced here, where Partitions = Array[LocalPartitions[T]] and LocalPartitions = List.

    def mutateRandomRecord(mutate: T => T): Partitions[T] = {
      val (partitionIndex, indexWithinPartition) = randomRecordIndex()
      val newElement: T = mutate(partitions(partitionIndex)(indexWithinPartition))

      val newPartition: LocalPartition[T] = partitions(partitionIndex).updated(
        indexWithinPartition, newElement
      ).toLocalPartition

      partitions.updated(partitionIndex, newPartition).toArray[LocalPartition[T]].toPartitions
     */


    partitions.mutateRandomRecord(this.mutateValue)

  }

  def mutateValue(input: T): T
}

abstract class StringSubstringReplacementMutationFn extends RandomRecordMutationFn[String] {
  private val _mutateRecord = TypeFuzzingUtil.mutateStrBySubstring(generateSubstringReplacement)
  override final def mutateValue(input: String): String = {
    _mutateRecord(input)
  }

  def generateSubstringReplacement(orig: String): String
}

/** Base mutation function for String-types: replaces a random substring with a newly generated random substring. */
case class GenericStringMutationFn(minLength: Int = TypeFuzzingUtil.MIN_STRING_SUB_LENGTH,
                              maxLength: Int = TypeFuzzingUtil.MAX_STRING_SUB_LENGTH) extends StringSubstringReplacementMutationFn {
  override def generateSubstringReplacement(orig: String): String = {
    TypeFuzzingUtil.randomString(minLength, maxLength)
  }
}

case class GenericIntMutationFn(min: Int = TypeFuzzingUtil.DEFAULT_INT_MIN, max: Int = TypeFuzzingUtil.DEFAULT_INT_MAX) extends RandomRecordMutationFn[Int] {
  override def mutateValue(input: Int): Int = {
    TypeFuzzingUtil.randomIntInRange(min, max)
  }
}

case class GenericBooleanMutationFn() extends RandomRecordMutationFn[Boolean] {
  override def mutateValue(input: Boolean): Boolean = {
    TypeFuzzingUtil.randBoolean()
  }
}

/** Base class for key-specific mutations.
  * TABLE MAPPING: ReplaceTupleElement */
class RandomKeyMutationFn[K: ClassTag, V: ClassTag](keyMutation: K => K) extends RandomRecordMutationFn[(K, V)] {
  override def mutateValue(input: (K, V)): (K, V) = {
    input.copy(_1 = keyMutation(input._1))
  }
}

/** Generic key mutation class relying on [[TypeFuzzingUtil.genericValueMutator()]] */
case class GenericRandomKeyMutationFn[K: ClassTag, V: ClassTag]()
  extends RandomKeyMutationFn[K, V](TypeFuzzingUtil.genericValueMutator[K]()) {
}

/** Base class for value-specific mutations.
  * TABLE MAPPING: ReplaceTupleElement*/
class RandomValueMutationFn[K: ClassTag, V: ClassTag](valueMutation: V => V) extends RandomRecordMutationFn[(K, V)] {
  override def mutateValue(input: (K, V)): (K, V) = {
    input.copy(_2 = valueMutation(input._2))
  }
}

/** Generic value mutation class relying on [[TypeFuzzingUtil.genericValueMutator()]] */
case class GenericRandomValueMutationFn[K: ClassTag, V: ClassTag]()
  extends RandomValueMutationFn[K, V](TypeFuzzingUtil.genericValueMutator[V]()) {
}

// TABLE MAPPING: AppendCollectionCopy
case class GenericValueArrayDuplMutationFn[K: ClassTag, V: ClassTag](duplFactor: Int = 2)
extends RandomValueMutationFn[K, Array[V]](
  // duplicate array by concatenating with itself
  if(duplFactor == 2) {
    // hardcode for 2-case for efficiency
    arr => arr ++ arr
  } else {
    arr => {
      // Previously tried: Seq.fill(...)(...).flatten.toArray - flatten operation is expensive
      // next tried replacing with Array.concat, but the initial Seq.fill can be expensive anyways.
      // Now just doing it manually.
      val arrLen = arr.length
      val newArrLen = arrLen * duplFactor
      //log(s"MEMDEBUG: Allocating array[$newArrLen]...")
      val result = Array.ofDim[V](newArrLen)
      //log("MEMDEBUG: Copying array...")
      (0 until duplFactor).foreach(idx =>
        Array.copy(arr, 0, result, idx * arrLen, arrLen)
      )
      //log("MEMDEBUG: Done copying array!")
      result
    }
  }
)

// TABLE MAPPING: AppendCollectionCopy
case class GenericIterableValueDuplMutationFn[K: ClassTag, V: ClassTag](duplFactor: Int = 2)
  extends RandomValueMutationFn[K, Iterable[V]](
    // duplicate array by concatenating with itself
    if(duplFactor == 2) {
      // hardcode for 2-case for efficiency?
      arr => arr ++ arr
    } else {
      arr => {
        // Previously tried: Seq.fill(...)(...).flatten.toArray - flatten operation is expensive
        // next tried replacing with Array.concat, but the initial Seq.fill can be expensive anyways.
        // Now just doing it manually.
        val arrLen = arr.size
        val newArrLen = arrLen * duplFactor
        //log(s"MEMDEBUG: Allocating array[$newArrLen]...")
        val result = Array.ofDim[V](newArrLen)
        //log("MEMDEBUG: Copying array...")
        (0 until duplFactor).foreach(idx =>
          Array.copy(arr, 0, result, idx * arrLen, arrLen)
        )
        //log("MEMDEBUG: Done copying array!")
        result
      }
    }
  )

// TABLE MAPPING: ReplaceCollectionElement
class IterableValueMutationFn[K: ClassTag, V: ClassTag](valueFn: V => V)
  extends RandomValueMutationFn[K, Iterable[V]](trav => {
    // quick, inefficient implementation to replace one element with a mutation.
    val arr = trav.toArray
    val choiceIdx = TypeFuzzingUtil.randomIntInRange(0, arr.length)
    arr(choiceIdx) = valueFn(arr(choiceIdx))
    arr
  })

case class GenericIterableValueMutationFn[K: ClassTag, V: ClassTag]()
extends IterableValueMutationFn[K, V](TypeFuzzingUtil.genericValueMutator[V]())

object QuadrupleMutations {
  // TABLE MAPPING: ReplaceQuadrupleElement
  // Recommended to multi-edit or figure out a way to autogen these as they are very similar.

  // V1
  class RandomQuadrupleV1MutationFn[V1: ClassTag, V2: ClassTag, V3: ClassTag, V4: ClassTag](v1MutationFn: V1 => V1)
    extends RandomRecordMutationFn[(V1, V2, V3, V4)] {
    override def mutateValue(input: (V1, V2, V3, V4)): (V1, V2, V3, V4) = {
      input.copy(_1 = v1MutationFn(input._1))
    }
  }

  case class GenericRandomQuadrupleV1MutationFn[V1: ClassTag, V2: ClassTag, V3: ClassTag, V4: ClassTag]()
    extends RandomQuadrupleV1MutationFn[V1, V2, V3, V4](TypeFuzzingUtil.genericValueMutator[V1]())

  // V2
  class RandomQuadrupleV2MutationFn[V1: ClassTag, V2: ClassTag, V3: ClassTag, V4: ClassTag](v2MutationFn: V2 => V2)
    extends RandomRecordMutationFn[(V1, V2, V3, V4)] {
    override def mutateValue(input: (V1, V2, V3, V4)): (V1, V2, V3, V4) = {
      input.copy(_2 = v2MutationFn(input._2))
    }
  }

  case class GenericRandomQuadrupleV2MutationFn[V1: ClassTag, V2: ClassTag, V3: ClassTag, V4: ClassTag]()
    extends RandomQuadrupleV2MutationFn[V1, V2, V3, V4](TypeFuzzingUtil.genericValueMutator[V2]())

  // V3
  class RandomQuadrupleV3MutationFn[V1: ClassTag, V2: ClassTag, V3: ClassTag, V4: ClassTag](v3MutationFn: V3 => V3)
    extends RandomRecordMutationFn[(V1, V2, V3, V4)] {
    override def mutateValue(input: (V1, V2, V3, V4)): (V1, V2, V3, V4) = {
      input.copy(_3 = v3MutationFn(input._3))
    }
  }

  case class GenericRandomQuadrupleV3MutationFn[V1: ClassTag, V2: ClassTag, V3: ClassTag, V4: ClassTag]()
    extends RandomQuadrupleV3MutationFn[V1, V2, V3, V4](TypeFuzzingUtil.genericValueMutator[V3]())

  // V4
  class RandomQuadrupleV4MutationFn[V1: ClassTag, V2: ClassTag, V3: ClassTag, V4: ClassTag](v4MutationFn: V4 => V4)
    extends RandomRecordMutationFn[(V1, V2, V3, V4)] {
    override def mutateValue(input: (V1, V2, V3, V4)): (V1, V2, V3, V4) = {
      input.copy(_4 = v4MutationFn(input._4))
    }
  }

  case class GenericRandomQuadrupleV4MutationFn[V1: ClassTag, V2: ClassTag, V3: ClassTag, V4: ClassTag]()
    extends RandomQuadrupleV4MutationFn[V1, V2, V3, V4](TypeFuzzingUtil.genericValueMutator[V4]())


}


/** Base class that exposes an endpoint to mutate a single random partition. By default, this class
  * will attempt to find a non-empty partition to mutate. If all partition are empty, this mutation
  * returns the original input.*/
abstract class RandomPartitionMutationFn[T: ClassTag] extends PartitionsBasedMutationFn[T] {
  override final def mutatePartitions(partitions: Partitions[T]): Partitions[T] = {
    val nonEmptyPartitions = partitions.zipWithIndex.filter({
      case (partition: LocalPartition[T], idx) =>
        partition.nonEmpty})
    if(nonEmptyPartitions.isEmpty) return partitions //

    val choice = TypeFuzzingUtil.randomChoice(nonEmptyPartitions)._2
    log(s"Selected partition #$choice")
    val origPartition = partitions(choice)
    /*
    val choice = TypeFuzzingUtil.randomIntInRange(0, partitions.length)
    val origPartition: LocalPartition[T] = partitions(choice)
    */
    val newPartition: LocalPartition[T] = this.mutatePartition(origPartition)
    // cast due to build errors.
    val result: Partitions[T] = partitions.updated(choice, newPartition).asInstanceOf[Partitions[T]]
    result
  }

  def mutatePartition(partition: LocalPartition[T]): LocalPartition[T]

  // helper function for subclasses
  protected def randomRecord(partition: LocalPartition[T]): T = {
    TypeFuzzingUtil.randomChoice(partition)
  }
}


/** Pick a random key and reuse it to append (generate) additional records with different values.
  * Up to `duplProportion` * partitionSize records will be added, with the actual number selected randomly.)
  * TABLEMAPPING: AppendSameKey
  */
class KeyDuplGenMutationFn[K: ClassTag, V: ClassTag](valueGenerator: V => V,
                                                     duplProportion: Double)
  extends RandomPartitionMutationFn[(K, V)] {
  override def mutatePartition(partition: LocalPartition[(K, V)]): LocalPartition[(K, V)] = {
    val (key, origValue) = randomRecord(partition)
    //println("DEBUG:" + partition.size)
    val maxDupes = Math.ceil(duplProportion * partition.size).toInt
    val numDupes = TypeFuzzingUtil.randomIntInRange(1, maxDupes + 1) // +1 because end range is exclusive.
    val newRecords = (1 to numDupes).map(_ => (key, valueGenerator(origValue)))
    partition ++ newRecords
  }
}

// Concrete class with existing/available classtag to facilitate inference.
case class GenericKeyDuplGenMutationFn[K: ClassTag, V: ClassTag](duplProportion: Double = 0.10) extends KeyDuplGenMutationFn[K, V](TypeFuzzingUtil.genericValueMutator[V](), duplProportion)

/** Identical to [[KeyDuplGenMutationFn]] except with key/value swapped.
  * TABLEMAPPING: AppendSameValue
  */
class ValueDuplGenMutationFn[K: ClassTag, V: ClassTag](keyGenerator: K => K,
                                                       duplProportion: Double)
  extends RandomPartitionMutationFn[(K, V)] {
  //logEnabled = true // temp override.
  override def mutatePartition(partition: LocalPartition[(K, V)]): LocalPartition[(K, V)] = {
    val (origKey, value) = randomRecord(partition)

    val maxDupes = Math.ceil(duplProportion * partition.size).toInt
    val numDupes = TypeFuzzingUtil.randomIntInRange(1, maxDupes + 1) // +1 because end range is exclusive.
    log(s"Adding $numDupes records out of potential max $maxDupes in partition of size ${partition.size} (* $duplProportion)")
    val newRecords = (1 to numDupes).map(_ => (keyGenerator(origKey), value))
    partition ++ newRecords
  }
}

// Concrete class with existing/available classtag to facilitate inference.
case class GenericValueDuplGenMutationFn[K: ClassTag, V: ClassTag](duplProportion: Double = 0.10) extends ValueDuplGenMutationFn[K, V](TypeFuzzingUtil.genericValueMutator[K](), duplProportion)

/**
 * Pick a random key and generate distinct records combining it with each value present in the partition.
 * This has the potential to drastically increase the number of values mapping to a particular key,
 * but it might also have no effect (e.g. for a very popular key) and is very generalized so may violate
 * some required application logic on key-value relationships.
 * TABLE MAPPING: PairKeyToAllValues
 */
case class GenericKeyEnumerationMutationFn[K: ClassTag, V: ClassTag]()
  extends RandomPartitionMutationFn[(K, V)] {
  override def mutatePartition(partition: LocalPartition[(K, V)]): LocalPartition[(K, V)] = {
    val (key, value) = randomRecord(partition) // value unused.
    val newRecords = partition.filterNot(_._1 == key) // don't need to duplicate anything for our existing key
                              .map(_._2) // extract the values
                              .distinct // deduplicate
                              .map((key, _)) // create new record with fixed key.
    partition ++ newRecords
  }
}

/**
 * Pick a random value and generate distinct records combining it with each key present in the partition.
 * This has the potential to drastically increase the number of keys mapping to a particular value,
 * but it might also have no effect (e.g. for a very popular value) and is very generalized so may violate
 * some required application logic on key-value relationships.
 * TABLE MAPPING: PairValueToAllKeys
 */
case class GenericValueEnumerationMutationFn[K: ClassTag, V: ClassTag]()
  extends RandomPartitionMutationFn[(K, V)] {
  override def mutatePartition(partition: LocalPartition[(K, V)]): LocalPartition[(K, V)] = {
    val (key, value) = randomRecord(partition) // key unused
    val newRecords = partition.filterNot(_._2 == value) // don't need to duplicate anything for our existing value
      .map(_._1) // extract the keys
      .distinct // deduplicate
      .map((_, value)) // create new record with fixed value.
    partition ++ newRecords
  }
}


/** Weight-based sampler that also supports the mutate operation (though it might be better to separate for debugging/clarity)
 * Currently outdated as of 7/12/2021. */
class WeightedMutationFnSelector[T](mutatorsWithWeights: Map[MutationFn[T], Double], rand: Random = Random)
  extends WeightedSampler[MutationFn[T]](mutatorsWithWeights, rand) with MutationFn[T] {

  logEnabled = false

  def selectMutator(): MutationFn[T] = sample() // alias

  override def mutate(input: HybridRDD[T]): HybridRDD[T] = {
    val (fn, mutation) = selectAndMutate(input)
    mutation
  }

  def selectAndMutate(input: HybridRDD[T]): (MutationFn[T], HybridRDD[T]) = {
    val mutator = selectMutator()
    log(s"Selected mutation function: $mutator")
    MutationFn.mostRecent = Some(mutator)
    (mutator, mutator.mutate(input))
  }
}

/** Weight-based sampler that also supports the mutate operation (though it might be better to separate for debugging/clarity) */
class WeightedPartitionMutationFnSelector[T](mutatorsWithWeights: Map[PartitionsBasedMutationFn[T], Double], rand: Random = Random)
  extends WeightedSampler[PartitionsBasedMutationFn[T]](mutatorsWithWeights, rand) with PartitionsBasedMutationFn[T] {

  logEnabled = false

  // Use weighted random sampling.
  def selectMutator(): PartitionsBasedMutationFn[T] = sample() // alias

  override def mutatePartitions(input: Partitions[T]): Partitions[T] = {
    val (fn, mutation) = selectAndMutate(input)
    mutation
  }


  def selectAndMutate(input: Partitions[T]): (PartitionsBasedMutationFn[T], Partitions[T]) = {
    val mutator = selectMutator()
    log(s"Selected partition mutation function: $mutator")
    MutationFn.mostRecent = Some(mutator)
    (mutator, mutator.mutatePartitions(input))
  }
}

object TypeFuzzingUtil extends HFLogger {
  val rand = Random
  val MAX_STRING_SUB_LENGTH = 25
  val MIN_STRING_SUB_LENGTH = 0

  // Note: MinValue means that Max-Min = -1, which results in an error
  // when selecting within range (might also be why default nextInt is in range [0, max)? )
  val DEFAULT_INT_MIN = 0
  val DEFAULT_INT_MAX = Int.MaxValue

  // TABLE MAPPING: ReplaceBoolean
  def randBoolean(): Boolean = {
    rand.nextBoolean()
  }

  /** Random integer in specified range [min, max). */
  def randomIntInRange(min: Int, max: Int): Int = {
    min + rand.nextInt(max - min)
  }

  /** Random double in specified range [min, max). */
  def randomDoubleInRange(min: Double, max: Double): Double = {
    min + (rand.nextDouble() * max - min)
  }

  def randomChoice[T](seq: Seq[T]): T = {
    seq(rand.nextInt(seq.length))
  }


  /** Generate random string.
    * Typically not used directly, instead you want to be able to mutate according to substring.
    * (See [[mutateStrBySubstring()]])
    */
  def randomString(minLength: Int = MIN_STRING_SUB_LENGTH, maxLength: Int = MAX_STRING_SUB_LENGTH) = {
    val replacementLength = randomIntInRange(minLength, maxLength)
    val replacementStr = rand.nextString(replacementLength)
    replacementStr
  }

  // TABLE MAPPING: ReplaceInteger
  def genericIntMutationFn(unused: Int): Int =
    randomIntInRange(DEFAULT_INT_MIN, DEFAULT_INT_MAX)


  // In the absence of any known bounds, we just default to the int range
  // TABLE MAPPING: ReplaceDouble
  def genericDoubleFn(unused: Double): Double =
    randomDoubleInRange(DEFAULT_INT_MIN, DEFAULT_INT_MAX)


  /** Mutate a string by replacing a random substring with a newly generated string (using the provided argument).
    * By default, the newly generated string is random (see [[randomString()]]
    * TABLE MAPPING: ReplaceSubstring
    */
  def mutateStrBySubstring(replacementStrFn: String => String = _ => randomString()): String => String = {
    s => {
      val strLen = s.length
      val startIndex = randomIntInRange(0, strLen + 1)
      val endIndex = startIndex + randomIntInRange(0, strLen - startIndex + 1)
      val replacementStr = replacementStrFn(s.substring(startIndex, endIndex))


      val initCapacity = startIndex + replacementStr.length + (strLen - endIndex)

      /*val prefix = s.substring(0, startIndex)
      val suffix = s.substring(endIndex)
      val builder = new StringBuilder(initCapacity, prefix)
      builder.append(replacementStr).append(suffix).toString()*/

      val builder = new StringBuilder(initCapacity, s)
      builder.delete(startIndex, endIndex)
      builder.insert(startIndex, replacementStr)
      val result = builder.toString()
      //println(s"$s => $result")
      result
    }
  }

  /** Generic functions for arbitrary values. Default mutations are configurable. */
  def genericValueMutator[T: ClassTag](strFn: String => String = mutateStrBySubstring(),
                                       intFn: Int => Int = genericIntMutationFn,
                                       doubleFn: Double => Double = genericDoubleFn,
                                       boolFn: Boolean => Boolean = _ => randBoolean()): T => T = {

    val result = classTag[T] match {
      case strTag if strTag == classTag[String] =>
        strFn
      case intTag if intTag == classTag[Int] =>
        intFn
      case doubleTag if doubleTag == classTag[Double] =>
        doubleFn
      case boolTag if boolTag == classTag[Boolean] =>
        boolFn
      case arrTag if arrTag.runtimeClass.isArray =>
        // Things are a bit trickier here, but checking for array is simple enough...
        // Problem is the underlying/nested type of the array.
        log(s"Unsupported tag for array inference. Defaulting to identity...: ${arrTag}")
        identity[T] _ // T => T

      case unknown =>
        val msg = s"Unsupported tag for genericValueMutator inference: ${classTag[T]}"
        log(msg)
        throw new UnsupportedOperationException(msg)
    }
    result.asInstanceOf[T => T]
  }
}
\end{lstlisting}
