# Supplementary material for: PerfGen: Automated Performance Benchmark Generation for Big Data Analytics
Source: arXiv:2412.04687 source file (2024-12-06)
Supplement: Supplementary file 3 [file mutation_maps.tex]

\begin{lstlisting}[language=Scala,label={appendix:mutation_maps}]
package edu.ucla.cs.hybridfuzz.phase.mutations

import edu.ucla.cs.hybridfuzz.metrictemplate.{MonitorTemplate, Metrics}
import edu.ucla.cs.hybridfuzz.util.HFLogger

import scala.collection.mutable
import scala.collection.mutable.ListBuffer
import scala.reflect.{ClassTag, classTag}

object MutationFnMaps extends HFLogger {

  // Note: current dev support is specifically for partition-based, rather than general mutation fns.
  type MutationMap[T] = Map[PartitionsBasedMutationFn[T], Double]
  // Temporary structure for creating finalized maps.
  type MutableMutationMap[T] = mutable.Map[PartitionsBasedMutationFn[T], Double]

  // Mutation maps for base data types.
  def getBaseMap[T: ClassTag](strMap: MutationMap[String] = Map(GenericStringMutationFn() -> 1.0),
                              intMap: MutationMap[Int] = Map(GenericIntMutationFn() -> 1.0),
                              boolMap: MutationMap[Boolean] = Map(GenericBooleanMutationFn() -> 1.0)): MutationMap[T] = {
    val result = classTag[T] match {
      case strTag if strTag == classTag[String] =>
        strMap
      case intTag if intTag == classTag[Int] =>
        intMap
      case boolTag if boolTag == classTag[Boolean] =>
        boolMap
      case arrTag if arrTag.runtimeClass.isArray =>
        // Things are a bit trickier here, but checking for array is simple enough...
        null

      case unknown =>
        log(s"Unsupported tag for genericValueMutator inference: ${classTag[T]}")
        null
    }
    result.asInstanceOf[MutationMap[T]]
  }

  // helper
  private def tryAppend[T](mutationFn: => PartitionsBasedMutationFn[T],
                              weight: Double,
                              name: String,
                              mutations: MutableMutationMap[T]): Unit = {
    try {
      mutations += (mutationFn -> weight)
    }catch {
      case e: Exception =>
        log(s"Unable to include mutation: $name")
        e.printStackTrace()
    }
  }

  /** Constructs map of tuple-based mutations with equal weight.*/
  def getTupleMap[K: ClassTag, V: ClassTag](duplGenProportion: Double = 0.10,
                                            keyMutationEnabled: Boolean = true,
                                            valueMutationEnabled: Boolean = true,
                                            template: Option[MonitorTemplate] = None,
                                            weighted: Boolean = true,
                                            uniqueKeys: Boolean = false
                                           ): MutationMap[(K, V)] = {
    if(uniqueKeys) throw new UnsupportedOperationException("Unique keys in getTupleMap not yet supported")
    // TODO: Future work: Incorporate uniqueKeys flag! (Should disable enumerations and key-duplication).
    // Currently it's not required.
    // note: it's technically possible, though unlikely, that value-duplication will result in a duplicate key.

    // Tuple-based functions have some options:
    // 1: Generic tuple mutation - mutate one or both fields randomly. This relies on
    // The classtags of the key and value to generate default values.
    // 2+3: Combine a key (or value) with every value (or key) in the partition.
    // 4+5: Add additional records belonging to a key or value, but with 'new' mutated keys/values (based on an existing key/value).
    val mutationMap: MutableMutationMap[(K, V)] = mutable.Map()

    if(template.isEmpty) throw new IllegalArgumentException("Jason: Templates required for evaluations now.")
    val isDataSkew = template.exists(_.metric.isDataSkew)
    val isRuntimeSkew = template.exists(_.metric.isRuntimeSkew)
    // Rule-based weight assignment:
    // if data skew, then it helps to increase the number of keys/values. Random typically only affects by one while
    // enumeration is capped and 'balanced' (i.e., not useful running multiple times), so upweight the duplications
    // even more than usual.
    val fixedDuplicationWeight =
      if(isDataSkew && weighted) 5.0
      else if (isRuntimeSkew && weighted) 3.0
      else 1.0

    // configure according to symptoms/templates,
    // e.g comp skew is more value-focused vs data skew more key-focused
    // deprecated in favor of smaller/more precise field mutations: tryAppend(GenericTupleMutationFn(), 1.0, "generic tuple mutation fn", mutationMap)
    if(keyMutationEnabled) {
      log("Key mutations enabled!")
      tryAppend(GenericRandomKeyMutationFn[K,V](), 1.0, "generic key mutation", mutationMap)

      // Note: This means fixed value and altered keys (duplicated value)
      tryAppend(GenericValueEnumerationMutationFn[K, V](), 1.0, "generic value enum fn", mutationMap)
      tryAppend(GenericValueDuplGenMutationFn[K, V](duplGenProportion), fixedDuplicationWeight, "generic value duplication", mutationMap)

    }

    if(valueMutationEnabled) {
      log("Value mutations enabled!")
      tryAppend(GenericRandomValueMutationFn[K, V](), 1.0, "generic value mutation", mutationMap)

      // Note: This means fixed key and altered values
      tryAppend(GenericKeyEnumerationMutationFn[K, V](), 1.0, "generic key enum fn", mutationMap)
      tryAppend(GenericKeyDuplGenMutationFn[K, V](duplGenProportion), fixedDuplicationWeight, "generic key duplication", mutationMap)
    }


    mutationMap.toMap
  }

  /** A specialized version of TupleMap used only for RQ3 and DeptGPAsQuartiles.
    * The objective here is to experiment with different weights of mutations, so
    * they have been parameterized.
    * */
  def getTupleMapRQ3DeptGPAsQuartiles[K: ClassTag, V: ClassTag](
                                                                 fixedDuplicationWeight: Double,
                                                                 duplGenProportion: Double = 0.10,
                                                                 keyMutationEnabled: Boolean = true,
                                                                 valueMutationEnabled: Boolean = true,
                                                                 template: Option[MonitorTemplate] = None,
                                                                 weighted: Boolean = true,
                                                                 uniqueKeys: Boolean = false,
                                           ): MutationMap[(K, V)] = {
    if(uniqueKeys) throw new UnsupportedOperationException("Unique keys in getTupleMap not yet supported")
    // TODO: Future work: Incorporate uniqueKeys flag! (Should disable enumerations and key-duplication).
    // Currently it's not required.
    // note: it's technically possible, though unlikely, that value-duplication will result in a duplicate key.

    // Tuple-based functions have some options:
    // 1: Generic tuple mutation - mutate one or both fields randomly. This relies on
    // The classtags of the key and value to generate default values.
    // 2+3: Combine a key (or value) with every value (or key) in the partition.
    // 4+5: Add additional records belonging to a key or value, but with 'new' mutated keys/values (based on an existing key/value).
    val mutationMap: MutableMutationMap[(K, V)] = mutable.Map()

    if(template.isEmpty) throw new IllegalArgumentException("Jason: Templates required for evaluations now.")
    val isDataSkew = template.exists(_.metric.isDataSkew)
    val isRuntimeSkew = template.exists(_.metric.isRuntimeSkew)

    //Removed: fixedDuplicationWeight is now determined by parameter.

    // configure according to symptoms/templates,
    // e.g comp skew is more value-focused vs data skew more key-focused
    // deprecated in favor of smaller/more precise field mutations: tryAppend(GenericTupleMutationFn(), 1.0, "generic tuple mutation fn", mutationMap)
    if(keyMutationEnabled) {
      log("Key mutations enabled!")
      tryAppend(GenericRandomKeyMutationFn[K,V](), 1.0, "generic key mutation", mutationMap)

      // Note: This means fixed value and altered keys (duplicated value)
      tryAppend(GenericValueEnumerationMutationFn[K, V](), 1.0, "generic value enum fn", mutationMap)
      tryAppend(GenericValueDuplGenMutationFn[K, V](duplGenProportion), fixedDuplicationWeight, "generic value duplication", mutationMap)

    }

    if(valueMutationEnabled) {
      log("Value mutations enabled!")
      tryAppend(GenericRandomValueMutationFn[K, V](), 1.0, "generic value mutation", mutationMap)

      // Note: This means fixed key and altered values
      tryAppend(GenericKeyEnumerationMutationFn[K, V](), 1.0, "generic key enum fn", mutationMap)
      tryAppend(GenericKeyDuplGenMutationFn[K, V](duplGenProportion), fixedDuplicationWeight, "generic key duplication", mutationMap)
    }


    mutationMap.toMap
  }

  // Not used in any benchmarks.
  def getQuadrupleMap[V1: ClassTag, V2: ClassTag, V3: ClassTag, V4: ClassTag]: MutationMap[(V1, V2, V3, V4)] ={
    type Quadruple = (V1, V2, V3, V4)
    val mutationMap: MutableMutationMap[(V1, V2, V3, V4)] = mutable.Map()

    import QuadrupleMutations._
    tryAppend(GenericRandomQuadrupleV1MutationFn[V1, V2, V3, V4](), 1.0, "generic V1 mutation fn", mutationMap)
    tryAppend(GenericRandomQuadrupleV2MutationFn[V1, V2, V3, V4](), 1.0, "generic V2 mutation fn", mutationMap)
    tryAppend(GenericRandomQuadrupleV3MutationFn[V1, V2, V3, V4](), 1.0, "generic V3 mutation fn", mutationMap)
    tryAppend(GenericRandomQuadrupleV4MutationFn[V1, V2, V3, V4](), 1.0, "generic V4 mutation fn", mutationMap)


    mutationMap.toMap
  }

  // Not used in any benchmarks.
  def getTupleMapWithArrayValue[K: ClassTag, V: ClassTag]: MutationMap[(K, Array[V])] = {
    type ArrV = Array[V]
    val mutationMap: MutableMutationMap[(K, ArrV)] = mutable.Map()

    // configure according to symptoms/templates,
    // e.g comp skew is more value-focused vs data skew more key-focused
    // tryAppend(GenericTupleMutationFn(), 1.0, "generic tuple mutation fn", mutationMap)
    tryAppend(GenericRandomKeyMutationFn[K, ArrV](), 1.0, "generic key mutation", mutationMap)
    // Due to classtag limitations, arrays need to be handled separately
    // Heuristic assignment: array values need to be explored more frequently, so increase weight.
    tryAppend(GenericValueArrayDuplMutationFn[K, V](10), 5.0, "generic value array dupl", mutationMap)
    tryAppend(GenericKeyEnumerationMutationFn[K, ArrV](), 1.0, "generic key enum", mutationMap)
    tryAppend(GenericValueEnumerationMutationFn[K, ArrV](), 1.0, "generic value enum", mutationMap)


    mutationMap.toMap
  }

  // Collatz uses this with (Int, Iterable[Int])
  def getTupleMapWithIterableValue[K: ClassTag, V: ClassTag](template: Option[MonitorTemplate] = None,
                                                             duplGenProportion: Double = 0.10,
                                                             keyMutationEnabled: Boolean = true,
                                                             valueMutationEnabled: Boolean = true,
                                                             weighted: Boolean = true,
                                                             uniqueKeys: Boolean = false
                                                            ): MutationMap[(K, Iterable[V])] = {
    type IterV = Iterable[V]
    val mutationMap: MutableMutationMap[(K, IterV)] = mutable.Map()
    // uniqueKeys disables enumerations and key-duplication (key dupe not yet supported for iterable values though)
    // note: it's technically possible, though unlikely, that value-duplication will result in a duplicate key.

    // configure according to symptoms/templates,
    // e.g comp skew is more value-focused vs data skew more key-focused
    // if we're dealing with data or memory skew enumerations are more valuable in increasing record mapings/consumption at a time
    val isDataSkew = template.exists(_.metric.isDataSkew)
    val isRuntimeSkew = template.exists(_.metric.isRuntimeSkew)

    // Heuristically assigned weights.
    val enumerationWeight = if (isDataSkew) 3.0 else 0.5
    val fixedDuplicationWeight = 1.0

    if(keyMutationEnabled) {
      tryAppend(GenericRandomKeyMutationFn[K, IterV](), 1.0, "generic key mutation", mutationMap)
      if(!uniqueKeys) {
        tryAppend(GenericValueEnumerationMutationFn[K, IterV](), enumerationWeight, "generic value enum", mutationMap)
      }

      tryAppend(GenericValueDuplGenMutationFn[K, IterV](duplGenProportion), fixedDuplicationWeight, "generic key duplication", mutationMap)
    }


    if(valueMutationEnabled) {
      tryAppend(GenericIterableValueDuplMutationFn[K, V](), 1.0, "generic iterable value dupl", mutationMap)
      tryAppend(GenericIterableValueMutationFn[K, V](),
        5.0, "derived single-value mutation function", mutationMap)
      if(!uniqueKeys) {
        tryAppend(GenericKeyEnumerationMutationFn[K, IterV](), enumerationWeight, "generic key enum", mutationMap)
      }



      // Disabled: It's difficult to define a way to randomly generate new values in this case when the values are iterables, as
      // that requires some sort of composition (e.g. valuedupl + valuemutation) that's not yet supported.
      //tryAppend(GenericKeyDuplGenMutationFn[K, V](duplGenProportion), fixedDuplicationWeight, "generic key duplication", mutationMap)
    }
    // Due to classtag limitations, arrays need to be handled separately
    //tryAppend(GenericValueArrayDuplMutationFn[K, V](10), 5.0, "generic value array dupl", mutationMap)

    mutationMap.toMap
  }

  /** Generic functions for arbitrary values. Not currently used in any benchmarks. */
  def genericValueMutationFn[T: ClassTag](strFn: MutationFn[String] = GenericStringMutationFn(),
                                       intFn: MutationFn[Int] = GenericIntMutationFn(),
                                       boolFn: MutationFn[Boolean] = GenericBooleanMutationFn()): MutationFn[T] = {
    val result = classTag[T] match {
      case strTag if strTag == classTag[String] =>
        strFn
      case intTag if intTag == classTag[Int] =>
        intFn
      case boolTag if boolTag == classTag[Boolean] =>
        boolFn
      case arrTag if arrTag.runtimeClass.isArray =>
      // Things are a bit trickier here, but checking for array is simple enough...
       log(s"Unsupported tag for array type inference: ${classTag[T]}")
       null

      case unknown =>
       log(s"Unsupported tag for genericValueMutator inference: ${classTag[T]}")
       null
    }
    result.asInstanceOf[MutationFn[T]]
  }
}

\end{lstlisting}
