# Supplementary material for: PerfGen: Automated Performance Benchmark Generation for Big Data Analytics
Source: arXiv:2412.04687 source file (2024-12-06)
Supplement: Supplementary file 4 [file monitor_templates.tex]

\begin{lstlisting}[language=Scala,label={appendix:monitor_templates}]
package edu.ucla.cs.hybridfuzz.metrictemplate

import edu.ucla.cs.hybridfuzz.observers.PerfMetricsListener.StageId
import edu.ucla.cs.hybridfuzz.observers.PerfMetricsStats
import edu.ucla.cs.hybridfuzz.phase.observers.SparkMetricsPhaseObserver.SparkJobStats
import edu.ucla.cs.hybridfuzz.rddhybrid.HybridRDD
import edu.ucla.cs.hybridfuzz.util.{ExecutionResult, HFLogger, RunConfig}
import org.apache.commons.math3.stat.descriptive.moment.{Mean, Skewness, StandardDeviation}
import org.apache.commons.math3.stat.descriptive.rank.{Max, Median}

import scala.collection.mutable
import scala.reflect.ClassTag


sealed trait MonitorTemplate extends HFLogger {
  val metric: Metric
  // Documentation Note:
  // type StageId = Int
  // (AppId, JobId, etc. are also integer)
  // PerfMetricsStats derived from PerfDebug, containing SparkListener performance metrics.
  // type SparkJobStats = Map[(AppId, JobId, StageId, PartitionId), PerfMetricsStats]

  // Optional stage specifier relative to the end of the program (a negative lookup index).
  def checkSymptoms(result: ExecutionResult, lastInput: HybridRDD[_], stat: SparkJobStats, targetStageReversedOrderIdOpt: Option[StageId]): SymptomResult

  // partition metric optional and only used for debugging.
  case class SymptomResult(meetsCriteria: Boolean, feedbackScore: Double, partitionMetrics: Array[Long] = Array())

  def criteriaStr: String
}

object MonitorTemplate {
  // IQROutlier
  def IQRTemplate(metric: Metric,
                  thresholdFactor: Double = 1.5, includeLowerBound: Boolean = false): IQRMonitorTemplate = {
    new IQRMonitorTemplate(metric, thresholdFactor, includeLowerBound)
  }

  // ErrorDetection
  def ErrorTemplate(errorMsgSubstring: String, underlying: MonitorTemplate): ErrorMonitorTemplate = {
    new ErrorMonitorTemplate(errorMsgSubstring, underlying)
  }

  // LeaveOneOutRatio
  def singleTaskAvgTemplate(metric: Metric,
                            minFactor: Double,
                            minValueThreshold: Long = 200): SingleTaskAvgMonitorTemplate = {
    new SingleTaskAvgMonitorTemplate(metric, minFactor, minValueThreshold)
  }

  // ZScore
  def maxZScoreThresholdMetricTemplate(metric: Metric,
                                          lowerBound: Option[Double] = None,
                                          upperBound: Option[Double] = Some(1.0)): MaxZScoreThresholdMonitorTemplate = {
    new MaxZScoreThresholdMonitorTemplate(metric, lowerBound, upperBound)
  }

  // ModZScore
  def maxModZScoreThresholdMetricTemplate(metric: Metric,
                                          lowerBound: Option[Double] = None,
                                          upperBound: Option[Double] = Some(1.0)): MaxModZScoreThresholdMonitorTemplate = {
    new MaxModZScoreThresholdMonitorTemplate(metric, lowerBound, upperBound)
  }

  // Skewness
  def skewThresholdTemplate(metric: Metric,
                            lowerBound: Option[Double] = None,
                            upperBound: Option[Double] = Some(1.0)): SkewnessThresholdMonitorTemplate = {
    new SkewnessThresholdMonitorTemplate(metric, lowerBound, upperBound)
  }

  // MaximumThreshold
  def simpleThresholdTemplate(metric: Metric,
        threshold: Long): SimpleThresholdMonitorTemplate = {
    new SimpleThresholdMonitorTemplate(metric, threshold)
  }

  // NextComparison
  def nextComparisonThresholdMetricTemplate(metric: Metric,
                                            factor: Double): NextComparisonThresholdMonitorTemplate = {
    new NextComparisonThresholdMonitorTemplate(metric, factor)
  }

}


/** Interface to simplify looking up metrics for a specific stage. */
sealed trait SpecifiedStageMonitorTemplate extends MonitorTemplate {

  protected var lastResult: ExecutionResult = _
  protected var lastInput: HybridRDD[_] = _


  private var warnCounter = 0

  override final def checkSymptoms(result: ExecutionResult, lastInput: HybridRDD[_], stats: SparkJobStats, targetStageReversedOrderIdOpt: Option[StageId]): SymptomResult = {
    this.lastResult = result
    this.lastInput = lastInput

    if (!result.isSuccess) {
      val (meetsCriteria, score) = checkError(result, lastInput)
      return SymptomResult(meetsCriteria, score)
    }

    val statValues: Iterable[PerfMetricsStats] = if(targetStageReversedOrderIdOpt.isDefined) {
      val targetStageReversedOrderId = targetStageReversedOrderIdOpt.get
      // _3 = stageId: idea is to get the ordered stage IDs in reverse and use targetStageReverseOrderId to index into it.
      val stageIds = stats.keys.map(_._3).toSeq.distinct.sorted(Ordering[StageId].reverse)
      val targetStageIdOption: Option[StageId]  = stageIds.lift(math.abs(targetStageReversedOrderId))
      if(targetStageIdOption.isEmpty) {
        val errorMsg = s"No stage corresponding to specified stage index $targetStageReversedOrderId was found: $stats"
        if(RunConfig.getActiveConfig.errorOnMissingSparkMetrics) {
          log("ERROR: " + errorMsg)
          throw new RuntimeException(errorMsg)
        } else {
          val warnFreq = RunConfig.getActiveConfig.warnFreqOnMissingSparkMetrics
          warnCounter = warnCounter + 1// % warnFreq
          if(warnCounter % warnFreq == 0) {
            log("WARN: " + errorMsg)
            log(s"WARN: The above message is printed every $warnFreq instances ($warnCounter so far)")
          }
          return SymptomResult(false, Double.MinValue) // can't find partition metrics
        }
      }
      val targetStageId = targetStageIdOption.get
      stats.filterKeys(_._3 == targetStageId).values
    } else {
      stats.values
    }
    // Use performance metric to extract appropriate values from PerfMetricsStats.
    val partitionMetrics: Array[Long] = metric.computeColl(statValues).toArray
    log(s"Computed metric: ${partitionMetrics.sorted.reverse.mkString(",")}")


    val (meetsCriteria, feedbackScore) = checkSymptoms(partitionMetrics)
    //if(meetsCriteria) {
    //  log(s"Criteria met with feedback score $feedbackScore for metrics: ${partitionMetrics.mkString(",")}")
    //}
    metric.clear() // clear metrics afterwards, to avoid unintended side effects
    SymptomResult(meetsCriteria, feedbackScore, partitionMetrics)
  }

  def checkError(result: ExecutionResult, lastInput: HybridRDD[_]): (Boolean, Double) = {
    (false, -1.0) // TODO: default feedback value.
  }

  // Simplified endpoint for subclasses to implement.
  def checkSymptoms(partitionMetrics: Array[Long]): (Boolean, Double)
}
// Checks for production of error with specified substring.
// feedback score: derived from underlying template, in this example an IQRMonitorTemplate
case class ErrorMonitorTemplate(val errorMsgSubstring: String,
                                 val underlying: MonitorTemplate) extends MonitorTemplate {
  override val metric: Metric = underlying.metric

  override def checkSymptoms(result: ExecutionResult, lastInput: HybridRDD[_], stat: SparkJobStats, targetStageReversedOrderIdOpt: Option[StageId]): SymptomResult = {
    if (!result.isSuccess) {
      val msg = result.error.get.getMessage
      val matched = msg.contains(errorMsgSubstring)
      if(matched) {
        SymptomResult(true, Double.MaxValue)
      } else {
        // wrong error message
        SymptomResult(false, Double.MinValue)
      }
    } else {
      val symptomResult = underlying.checkSymptoms(result, lastInput, stat, targetStageReversedOrderIdOpt)
      SymptomResult(false, symptomResult.feedbackScore, symptomResult.partitionMetrics)
    }

  }

  override def criteriaStr: String = s"produces an error containing message $errorMsgSubstring"
}

/** Monitor Template that monitors the specified metric according to the IQR range.
 * See https://en.wikipedia.org/wiki/Outlier#Tukey's_fences for details.
 */
case class IQRMonitorTemplate(
                         override val metric: Metric,
                         val thresholdFactor: Double = 1.5,
                         val includeLowerBound: Boolean = true
                       ) extends SpecifiedStageMonitorTemplate {
  override def checkSymptoms(partitionMetrics: Array[Long]): (Boolean, Double) = {
    // simple solution for now, but note that it's inefficient in that it sorts everything when we only need Q1 and Q3.
    // There's probably some improved approaches where you can use a median-finding algorithm three times to
    // find Q2 and then Q1/Q3, if it's ever necesary.
    val numPartitions = partitionMetrics.length

    if(numPartitions < 2) {
      return (false, 0.0) // no results to process because too few partitions
    }



    val sorted = partitionMetrics.sorted
    // Use ceil - 1
    val q1Index = Math.ceil(numPartitions * 0.25).toInt - 1
    val q3Index = Math.ceil(numPartitions * 0.75).toInt - 1
    val q1 = sorted(q1Index)
    val q3 = sorted(q3Index)

    val IQR = Math.max(q3 - q1, 1) // ensure that we don't deal with a divide-by-zero
    val highFactor = (sorted.last - q3).toDouble / IQR // max - q3
    val maxFactor = if(includeLowerBound) {
      val lowFactor = (q1 - sorted.head).toDouble / IQR // q1 - min
      Math.max(lowFactor, highFactor)
    } else highFactor


    (maxFactor >= thresholdFactor, maxFactor)
  }

  override def criteriaStr: String = s"contains any partition $metric that is at least $thresholdFactor IQR above Q3${if (includeLowerBound) " or below Q1"}."
}

// Checks the ratio between each partition and the average of remaining partitions after its removal.
case class SingleTaskAvgMonitorTemplate(
                                 override val metric: Metric,
                                 val minFactor: Double,
                                 val minValueThreshold: Long = 200L,
                                 ) extends SpecifiedStageMonitorTemplate {


  override def checkSymptoms(partitionMetrics: Array[Long]): (Boolean, Double) = {
    if(partitionMetrics.isEmpty) {
      return (false, 0.0) // no results to process.
    }
    // compute average for the entire set.
    val sum = partitionMetrics.sum
    val count = partitionMetrics.length


    // For each partition metric, compute the other-average and output the corresponding ratio.
    val partitionScores = partitionMetrics.map(partitionMetric => {
      val allOthersAvg = (sum - partitionMetric).toDouble / (count - 1)
      //(partitionMetrics, allOthersAvg)
      val ratio = if(partitionMetric <= minValueThreshold) {
        // we don't want to consider cases when the metric is below threshold, so we zero it out.
        //Double.NegativeInfinity
        0.0
      } else if(allOthersAvg == 0.0) {
        // divide-by-zero, so return infinity instead.
        Double.PositiveInfinity
      } else {
        partitionMetric.toDouble / allOthersAvg
      }
      (partitionMetric, allOthersAvg, ratio)
    })

    val (maxMetric, maxMetricOtherAvg, maxRatio) = partitionScores.maxBy(_._3)

    val meetsCriteria = maxRatio >= minFactor

    if(meetsCriteria) {
      log(f"Found partition metric with ratio $maxRatio%.2f, value $maxMetric > max($minValueThreshold, $minFactor * $maxMetricOtherAvg%.2f (($sum - $maxMetric) / $count - 1))")
    } else {
      // did not pass threshold check.
    }

    (meetsCriteria, maxRatio)
  }

  override def criteriaStr: String = s"has a single executor with metric $metric that is at least ${minFactor}x that of remaining average"
}

// Partial implementation to specify upper and lower bounds for some numerically computed feedback score.
abstract class BoundedThresholdMonitorTemplate(val lowerBound: Option[Double],
                                               val upperBound: Option[Double]
                                             ) extends SpecifiedStageMonitorTemplate {
  assert(lowerBound.isDefined || upperBound.isDefined, "At least one of upper/lower bound must be defined.")

  /** Compute the desired aggregation feedback score (e.g., max z-score). */
  def computeFeedback(partitionMetrics: Array[Long]): Double
  val feedbackDescription: String


  override final def checkSymptoms(partitionMetrics: Array[Long]): (Boolean, Double) = {
    val metricValue = computeFeedback(partitionMetrics)
    val belowRange = lowerBound.exists(metricValue <= _)
    val aboveRange = upperBound.exists(metricValue >= _)
    val outOfRange =  belowRange || aboveRange
    (outOfRange, metricValue)
  }


  private val lbStringOpt = upperBound.map(b => s"greater than or equal to $b")
  private val ubStringOpt = lowerBound.map(b => s"less than or equal to $b")


  override final lazy val criteriaStr: String = {
    val sb = new StringBuilder(s"has a $feedbackDescription ")
    ubStringOpt.foreach(sb.append)
    if (ubStringOpt.isDefined && lbStringOpt.isDefined) {
      sb.append(" or ")
    }
    lbStringOpt.foreach(sb.append)
    sb.append(".")
    sb.toString()
  }
}

// Internal optimized array wrapper to only allocate more memory when necessary.
private class ResizableArrayConverter[T, U: ClassTag]() extends HFLogger {
  private var reusable: Array[U] = _
  private var maxLength = -1
  private var lastLength = -1

  def data: Array[U] = reusable
  def currentLength: Int = lastLength
  /** Applies the converter function into the reusable array and returns the new array +
    * the valid prefix length (which is always equal to the input length) */
  def convert(input: Array[T], fn: T => U): (Array[U], Int) = {
    // Try to reuse an existing array if possible, rather than simply creating a new one each time.
    // Many of the apache math libraries have APIs for supporting this sort of sub-array definition.
    if(maxLength < input.length) {
      log(s"INCREASING LENGTH FROM $maxLength to ${input.length}")
      maxLength = input.length
      reusable = new Array[U](maxLength)
      maxLength = input.length
    }
    lastLength = input.length
    input.zipWithIndex.foreach({case (value, index) => reusable(index) = fn(value)})
    (data, currentLength)
  }


}
/** Internally maintains a double-array and extends as needed. Subclasses accept a double array and a specified length
  * (extra elements after the specified length should be ignored).
  */
sealed trait DoubleArrayTracker extends BoundedThresholdMonitorTemplate {
  private val reusable: ResizableArrayConverter[Long, Double] = new ResizableArrayConverter()

  /** Compute the metric on the provided array, using only the first 'length' values. */
  def computeMetric(partitionMetrics: Array[Double], length: Int): Double

  override final def computeFeedback(partitionMetrics: Array[Long]): Double = {

    val (doubleData, targetLength) = reusable.convert(partitionMetrics, _.toDouble)
    computeMetric(doubleData, targetLength)
  }


}

/** Computes the largest z-score from the provided metrics.
  * */
case class MaxZScoreThresholdMonitorTemplate(
                                                override val metric: Metric,
                                                override val lowerBound: Option[Double] = None,
                                                override val upperBound: Option[Double] = Some(3.5),
                                              ) extends BoundedThresholdMonitorTemplate(lowerBound, upperBound) with DoubleArrayTracker {
  private val absMedianDiffConverter = new ResizableArrayConverter[Double, Double]()
  val meanStat = new Mean() // for use with MeanAD if needed.
  val stdDevStat = new StandardDeviation()
  val maxStat = new Max()

  override def computeMetric(partitionMetrics: Array[Double], length: Int): Double = {
    val mean = meanStat.evaluate(partitionMetrics, 0, length)
    val stdDev = stdDevStat.evaluate(partitionMetrics, 0, length)
    val max = maxStat.evaluate(partitionMetrics, 0, length)

    val maxZScore = (max - mean) / stdDev
    maxZScore
  }

  override val feedbackDescription: String = "maximum z-score"
                                              }
/** Computes the largest modified z-score from the provided metrics.
  * The modified z-score uses the median absolute deviation, rather than
  * standard deviation.
  * */
case class MaxModZScoreThresholdMonitorTemplate(
                                   override val metric: Metric,
                                   override val lowerBound: Option[Double] = None,
                                   override val upperBound: Option[Double] = Some(3.5),
                                   ) extends BoundedThresholdMonitorTemplate(lowerBound, upperBound) with DoubleArrayTracker {
  // Some resources:
  // https://medium.com/analytics-vidhya/anomaly-detection-by-modified-z-score-f8ad6be62bac
  // https://www.statology.org/modified-z-score/
  //val meanStat = new Mean()
  //val stdStat = new StandardDeviation()
  private val absMedianDiffConverter = new ResizableArrayConverter[Double, Double]()
  val medianStat = new Median()
  val meanStat = new Mean() // for use with MeanAD if needed.
  val maxStat = new Max()
  val medianADScaleFactor = 1.4826 // https://en.wikipedia.org/wiki/Median_absolute_deviation
  val meanADScaleFactor = 1.253314 // https://www.ibm.com/docs/en/cognos-analytics/11.1.0?topic=terms-modified-z-score

  override def computeMetric(partitionMetrics: Array[Double], length: Int): Double = {
    val median = medianStat.evaluate(partitionMetrics, 0, length)
    val (medianDevs, _) = absMedianDiffConverter.convert(partitionMetrics, x => Math.abs(x - median))
    val medianAD = medianStat.evaluate(medianDevs, 0, length)

    val denominator = if (medianAD != 0.0) {
      medianADScaleFactor * medianAD
    } else {
      // technically this is undefined. It seems IBM Cognos Analytics opts to use the mean abs deviation here instead.
      // https://www.ibm.com/docs/en/cognos-analytics/11.1.0?topic=terms-modified-z-score
      val meanAD = meanStat.evaluate(medianDevs, 0, length)
      //log(s"Median absolute deviation is zero, using meanAD instead: $meanAD")
      meanADScaleFactor * meanAD
    }

    // Impl note: medianDevs is the absolute maxes, which means an abnormally low value might be the 'max' absolute dev.
    // This is why we still use the max value - median, despite repeating a calculation.
    val maxValue = maxStat.evaluate(partitionMetrics, 0, length)
    val maxModZScore = (maxValue - median)/denominator

    //log(f"ModZScore: $maxModZScore%.2f from ($median%.2f, $medianAD%.2f, $maxValue%.2f, $denominator%.2f): ${partitionMetrics.mkString(",")}")
    maxModZScore

  }

  override val feedbackDescription: String = "maximum modified z-score"
}

/** Computed based on the definition of Skewness: https://en.wikipedia.org/wiki/Skewness
  * Uses apache commons math3.
  * If provided, minValue is used to indicate that at least one value must exceed this before being accepted. (not impl)
  * Note: Personal experimentation indicates this is not reliable for small sample sizes! (online searches also indicate
  * it can fluctuate quite a bit at < 50 points)
  */
case class SkewnessThresholdMonitorTemplate(
                                   override val metric: Metric,
                                   override val lowerBound: Option[Double] = None,
                                   override val upperBound: Option[Double] = Some(1.0),
                                   //val minValue: Option[Long] = None
                                 ) extends BoundedThresholdMonitorTemplate(lowerBound, upperBound) with DoubleArrayTracker {
  val skewnessStat = new Skewness()

  override def computeMetric(partitionMetrics: Array[Double], length: Int): Double = {
    // skewnessStat.clear()
    val skewness: Double = skewnessStat.evaluate(partitionMetrics, 0, length)
    if(skewness.isNaN) {
      // edge case to consider, e.g., if all values are equal
      if (partitionMetrics.length < 3) {
        log("Skewness metric requires at least three data points. Skipping (defaulting to 0)")
      } else if (partitionMetrics.forall(_ == partitionMetrics.head)) {
        //log("Skewness NaN due to uniform values")
        // This is expected in some cases, e.g. GC
      } else {
        log("Unknown reason for NaN skewness. Defaulting to 0...")
        log(partitionMetrics.mkString(","))
      }
    }
    skewness
  }

  override val feedbackDescription: String = "skewness metric"
}

/** Checks if the largest metric meets or exceeds the specified threshold. */
case class SimpleThresholdMonitorTemplate(override val metric: Metric,
                                          val threshold: Long
                                     ) extends BoundedThresholdMonitorTemplate(None, Some(threshold)) {

  override def computeFeedback(partitionMetrics: Array[Long]): Double = partitionMetrics.max

  override val feedbackDescription: String = "maximum value"
}

/** Checks if the ratio between the max and second-largest values is greater than the specified factor. */
case class NextComparisonThresholdMonitorTemplate(override val metric: Metric,
                                                  val factor: Double) extends BoundedThresholdMonitorTemplate(None, Some(factor)) {
  assert(factor > 1.0, "Factor must be at least one (i.e., at least 1x the next greatest value)")

  val minHeap = new mutable.PriorityQueue[Long]()(Ordering[Long].reverse)
  val maxSize = 2
  /** Compute the desired aggregation metric (e.g., max z-score). */
  override def computeFeedback(partitionMetrics: Array[Long]): Double = {
    if(partitionMetrics.length < maxSize) throw new IllegalArgumentException(s"Partition metrics too small: ${partitionMetrics.length}")
    partitionMetrics.foreach(value => {
      if(minHeap.size < maxSize) {
        minHeap.enqueue(value)
      } else if (minHeap.head < value) {
        minHeap.enqueue(value)
        minHeap.dequeue()
      }
    })

    val values = minHeap.dequeueAll
    val secondMax = values(0)
    val max = values(1)
    val factor = max.toDouble / secondMax
    factor
  }

  override val feedbackDescription: String = "ratio between largest and second largest value"
}
\end{lstlisting}
